# Supplementary material for: Dividing and Conquering a BlackBox to a Mixture of Interpretable Models: Route, Interpret, Repeat
Source: arXiv:2307.05350 source file (2023-07-12)
Supplement: Supplementary file 1 [file explanation_validity.tex]

To validate the concepts using the extracted FOL explanations, we intervene on the concepts in the derived FOL by setting the values of those concepts to zero for each sample. For example, the FOL explanation of instances in expert4 for the class ``Bay Breasted Warbler'' include concepts \st \emph{back\_pattern\_stripped} and \emph{leg\_color\_grey} in~\cref{fig:local_ex_cub}. For intervention, we set the values of these concepts to zero while values of other concepts remain unchanged. Next we pass the complete intervened concept vector as input to the associated expert, compute the
  performance and summarize the results in~\cref{tab:cf_table}. We discover that MoIE is highly susceptible to such interventions, and its performance drops significantly. For example,
  the performance of MoIE deteriorates from 0.91 to 0.42 \% (a 53.8 \% drop) for CUB-200 VIT-derived MoIE. 
  We compare the results with 1) the CBM + ELL baseline corresponding to CUB-200 (both Resnet101 and VIT), Awa2 (both Resnet101 and VIT) and Effusion of MIMIC-CXR; 2) PCBM + ELL baseline for the skin datasets. For CUB-200 VIT-based baseline model, the performance of the baseline drops by 26.5 \% drop, from 0.90 to 0.66. We observe a similar trend for other datasets as well. As MoIE selects more concrete, instance specific concepts than the baseline by covering subsets of data using various experts, its performance degrades severely compared to the baseline. 
  
\begin{table*}[h]
\caption{Validating the concepts purely by extracted FOL rules from MoIE and the baselines. Performance using original explanation refers to the performance of the model employing the concepts from the FOL explanations per sample. We intervene with these concepts by setting their values to zero and reporting it as ``Performance using intervened explanation'' in the table. In addition, we also show the drop in performance for the two scenarios. The larger drop in performance illustrates the model to be more sensitive to such intervention of the derived concepts.}\smallskip
\fontsize{6.75pt}{0.30cm}
\selectfont
\centering
\begin{tabular}{p{2.7em} c c c c c c c}
\toprule 
        \textbf{Model} & \multicolumn{7}{c}{\textbf{Performance using original explanation $\longrightarrow$ Performance using intervened explanation (drop \% )}} \\
       & CUB-200 (ResNet101) & CUB-200 (VIT )& Awa2 (ResNet101) & Awa2 (VIT) & HAM 10000 & ISIC  
       & Effusion\\
\midrule 
    MoIE & 
        0.88 $\rightarrow$ 0.65 (\textbf{26.1}) & 
        0.91 $\rightarrow$ 0.42 (\textbf{53.8}) & 
        0.87 $\rightarrow$ 0.54 (\textbf{37.9}) & 
        0.97 $\rightarrow$ 0.90 (\textbf{7.2})  & 
        0.95 $\rightarrow$ 0.92 (\textbf{3.1})  & 
        0.82 $\rightarrow$ 0.79 (\textbf{3.6})  &
        0.87 $\rightarrow$ 0.82 (\textbf{5.7}) 
    \\
\midrule 
    Baseline & 
        0.71 $\rightarrow$ 0.56 (\textbf{21.1}) & 
        0.90 $\rightarrow$ 0.66 (\textbf{26.5}) & 
        0.86 $\rightarrow$ 0.56 (\textbf{34.8}) & 
        0.94 $\rightarrow$ 0.92 (\textbf{2.1}) & 
        0.94 $\rightarrow$ 0.92 (\textbf{2.1}) &
        0.83 $\rightarrow$ 0.80 (\textbf{3.6}) &
        0.73 $\rightarrow$ 0.72 (\textbf{1.3})
        \\
\bottomrule
\end{tabular}
\label{tab:cf_table}
\end{table*}
