# Supplementary material for: Dividing and Conquering a BlackBox to a Mixture of Interpretable Models: Route, Interpret, Repeat
Source: arXiv:2307.05350 source file (2023-07-12)
Supplement: Supplementary file 3 [file performance_drop_other_v1.tex]

\begin{figure}
\centering
\includegraphics[width=\columnwidth]
{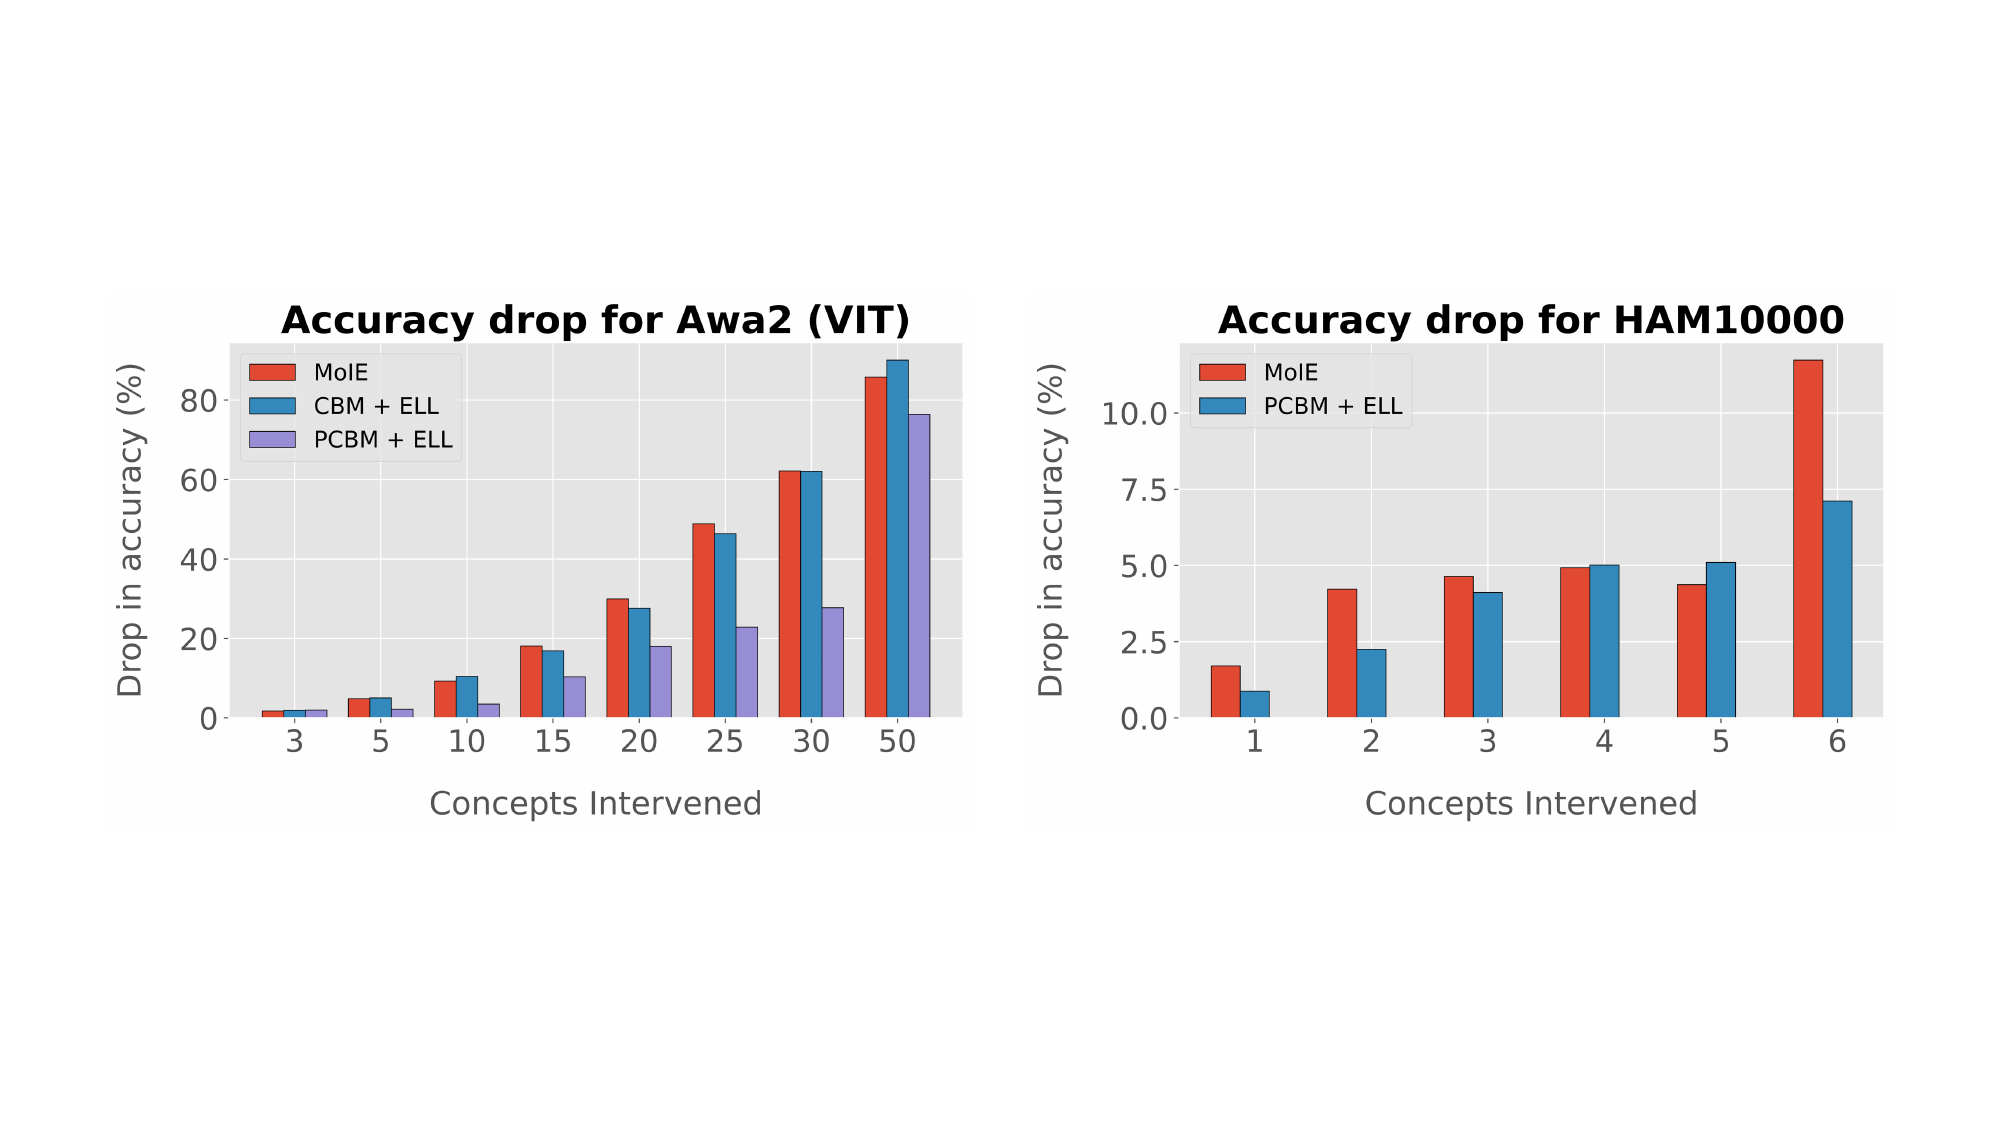}
\vskip -7pt
\caption{Validation of the concepts utilized for Awa2 (left) and HAM10000 (right) datasets by Inception and VIT-derived MoIE and the baselines respectively.}
\vskip -10pt
\label{fig:valid_concepts_other}
\end{figure}

\cref{fig:valid_concepts_other} shows the performance drop for HAM10000 and Awa2 when we intervene and set the values of the important concepts as zeros.
