# Supplementary material for: Dividing and Conquering a BlackBox to a Mixture of Interpretable Models: Route, Interpret, Repeat
Source: arXiv:2307.05350 source file (2023-07-12)
Supplement: Supplementary file 4 [file tti_v1.tex]

\begin{figure}
\centering
\includegraphics[width=\columnwidth]{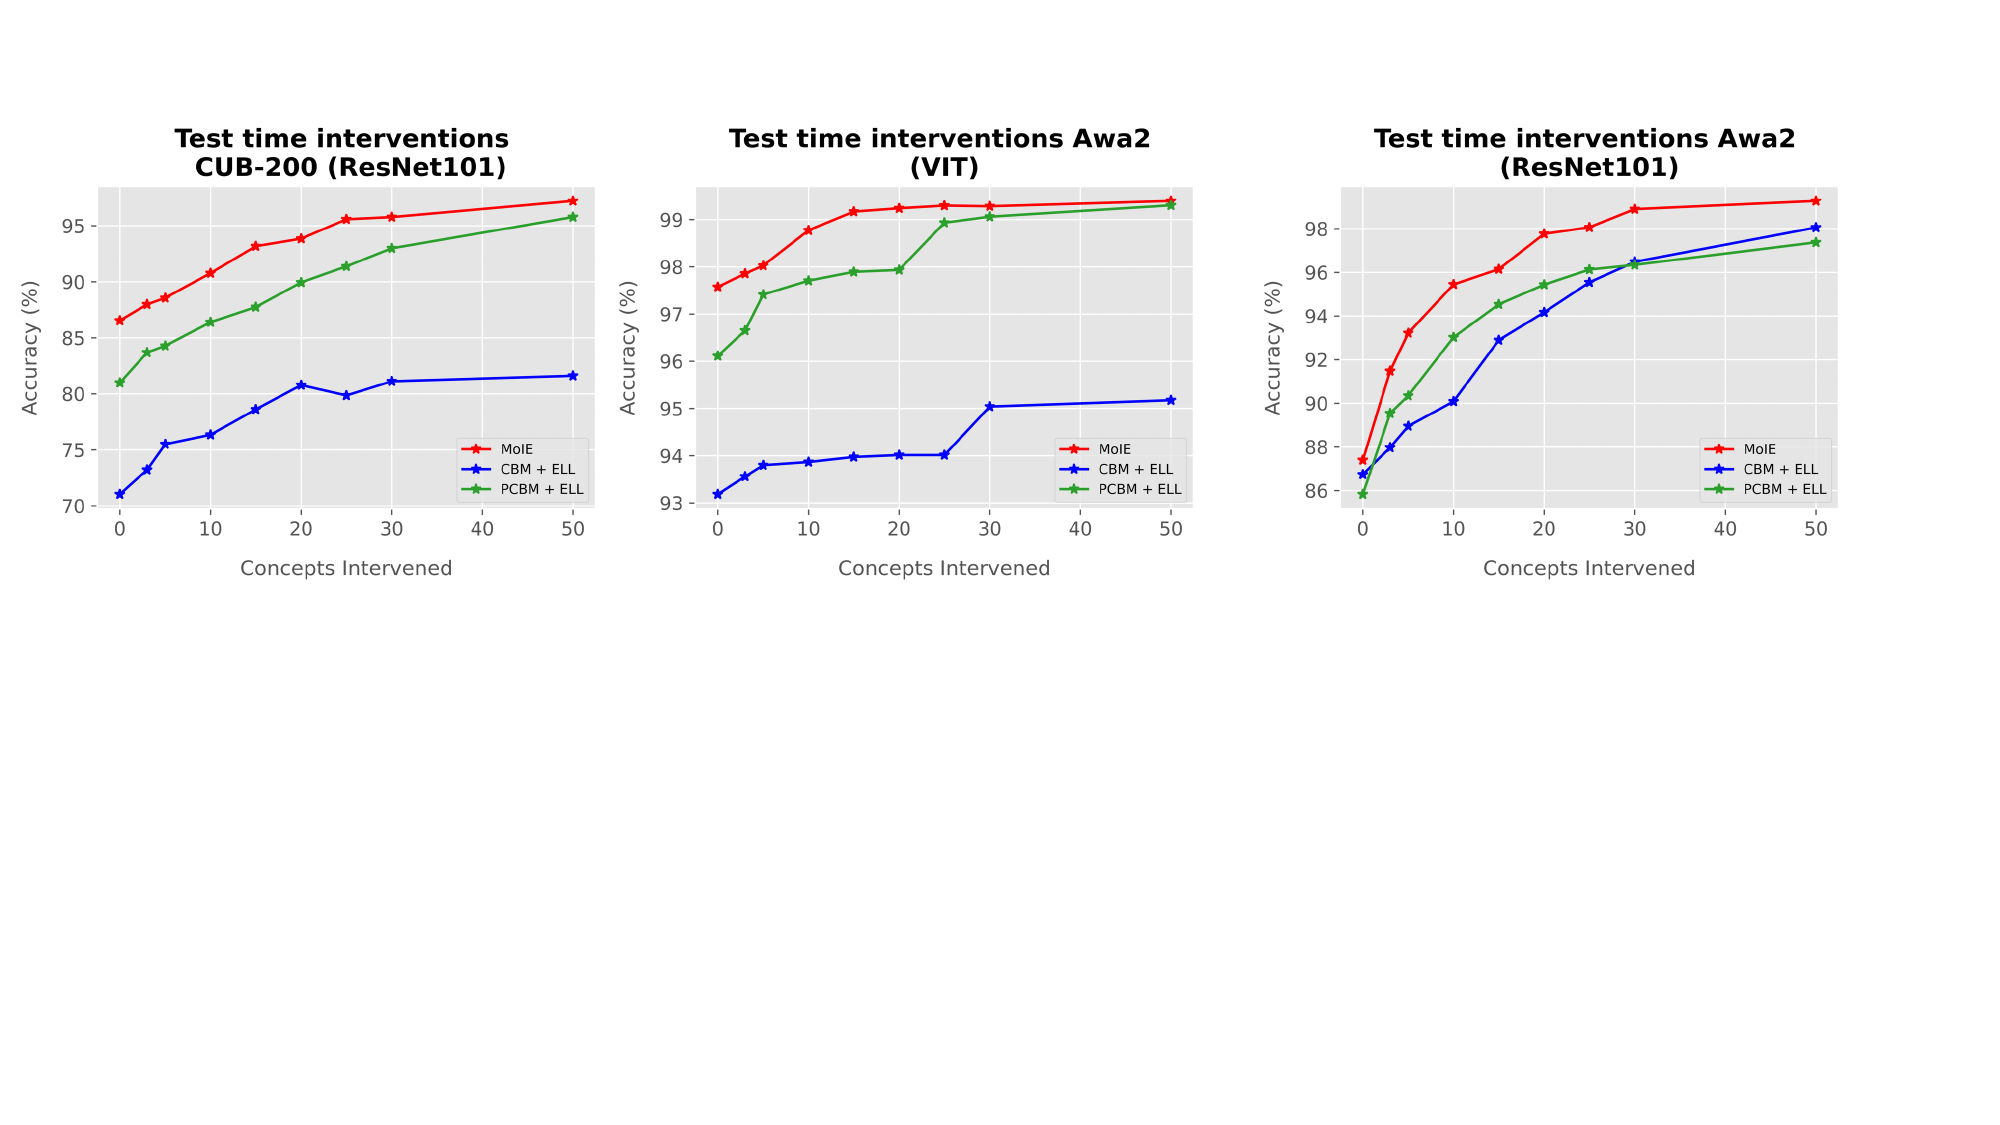}
\vskip -7pt
\caption{Illustration of test time interventions for ResNet101-derived models for CUB-200 (left) and VIT-derived models for Awa2 (middle) and ResNet101-driven models for Awa2 (right).}
\vskip -7pt
\label{fig:tti_expert}
\end{figure}

Figure~\ref{fig:tti_expert} shows the results of test time concept interventions for ResNet101-derived models for CUB-200 (left) and VIT-derived models for Awa2 (middle) and ResNet101-driven models for Awa2 (right).
